# Supplementary material for: Differential Privacy and Byzantine Resilience in SGD: Do They Add Up?
Source: arXiv:2102.08166 source file (2021-06-24)
Supplement: Supplementary file 1 [file experiments-appendix.tex]

\section{Experimental Results: Additional Settings}
\label{sec:exp-results-more}

This section completes the observations of Section \ref{sec:exp-results} by reporting on a larger set of training settings.
In particular, this section also reports on variations of the privacy constant $\epsilon$.
The range of tested values for $\epsilon$ and $b$ consists in every combination of: $\left( \epsilon, b \right) \in \left\lbrace 0.5, 0.2, 0.1 \right\rbrace \times \left\lbrace 10, 25, 50, 100, 250, 500 \right\rbrace$.
The results are reported from Fig.\ \ref{fig:experiments-more-10} to Fig.\ \ref{fig:experiments-more-500}.

\begin{figure}
    \centering
    \makebox[0.25\linewidth][c]{\footnotesize{}Without privacy noise}%
    \makebox[0.25\linewidth][c]{\footnotesize{}With privacy noise ($\epsilon = 0.5$)}%
    \makebox[0.25\linewidth][c]{\footnotesize{}With privacy noise ($\epsilon = 0.2$)}%
    \makebox[0.25\linewidth][c]{\footnotesize{}With privacy noise ($\epsilon = 0.1$)}\\[0.1mm]%
    \includeplot{0.25\linewidth}{e_inf-b_10}%
    \includeplot{0.25\linewidth}{e_0.5-b_10}\\%
    \includeplot{0.25\linewidth}{e_0.2-b_10}%
    \includeplot{0.25\linewidth}{e_0.1-b_10}\\%
    \includeplot{0.25\linewidth}{e_inf-b_10-loss}%
    \includeplot{0.25\linewidth}{e_0.5-b_10-loss}\\%
    \includeplot{0.25\linewidth}{e_0.2-b_10-loss}%
    \includeplot{0.25\linewidth}{e_0.1-b_10-loss}%
    \caption{In this set of experiments, the training batch size is $b = 10$.}
    \label{fig:experiments-more-10}
\end{figure}

\begin{figure}
    \centering
    \makebox[0.25\linewidth][c]{\footnotesize{}Without privacy noise}%
    \makebox[0.25\linewidth][c]{\footnotesize{}With privacy noise ($\epsilon = 0.5$)}%
    \makebox[0.25\linewidth][c]{\footnotesize{}With privacy noise ($\epsilon = 0.2$)}%
    \makebox[0.25\linewidth][c]{\footnotesize{}With privacy noise ($\epsilon = 0.1$)}\\[0.1mm]%
    \includeplot{0.25\linewidth}{e_inf-b_25}%
    \includeplot{0.25\linewidth}{e_0.5-b_25}\\%
    \includeplot{0.25\linewidth}{e_0.2-b_25}%
    \includeplot{0.25\linewidth}{e_0.1-b_25}\\%
    \includeplot{0.25\linewidth}{e_inf-b_25-loss}%
    \includeplot{0.25\linewidth}{e_0.5-b_25-loss}\\%
    \includeplot{0.25\linewidth}{e_0.2-b_25-loss}%
    \includeplot{0.25\linewidth}{e_0.1-b_25-loss}%
    \caption{In this set of experiments, the training batch size is $b = 25$.}
    \label{fig:experiments-more-25}
\end{figure}

\begin{figure}
    \centering
    \makebox[0.25\linewidth][c]{\footnotesize{}Without privacy noise}%
    \makebox[0.25\linewidth][c]{\footnotesize{}With privacy noise ($\epsilon = 0.5$)}%
    \makebox[0.25\linewidth][c]{\footnotesize{}With privacy noise ($\epsilon = 0.2$)}%
    \makebox[0.25\linewidth][c]{\footnotesize{}With privacy noise ($\epsilon = 0.1$)}\\[0.1mm]%
    \includeplot{0.25\linewidth}{e_inf-b_50}%
    \includeplot{0.25\linewidth}{e_0.5-b_50}\\%
    \includeplot{0.25\linewidth}{e_0.2-b_50}%
    \includeplot{0.25\linewidth}{e_0.1-b_50}\\%
    \includeplot{0.25\linewidth}{e_inf-b_50-loss}%
    \includeplot{0.25\linewidth}{e_0.5-b_50-loss}\\%
    \includeplot{0.25\linewidth}{e_0.2-b_50-loss}%
    \includeplot{0.25\linewidth}{e_0.1-b_50-loss}%
    \caption{In this set of experiments, the training batch size is $b = 50$.}
    \label{fig:experiments-more-50}
\end{figure}

\begin{figure}
    \centering
    \makebox[0.25\linewidth][c]{\footnotesize{}Without privacy noise}%
    \makebox[0.25\linewidth][c]{\footnotesize{}With privacy noise ($\epsilon = 0.5$)}%
    \makebox[0.25\linewidth][c]{\footnotesize{}With privacy noise ($\epsilon = 0.2$)}%
    \makebox[0.25\linewidth][c]{\footnotesize{}With privacy noise ($\epsilon = 0.1$)}\\[0.1mm]%
    \includeplot{0.25\linewidth}{e_inf-b_100}%
    \includeplot{0.25\linewidth}{e_0.5-b_100}\\%
    \includeplot{0.25\linewidth}{e_0.2-b_100}%
    \includeplot{0.25\linewidth}{e_0.1-b_100}\\%
    \includeplot{0.25\linewidth}{e_inf-b_100-loss}%
    \includeplot{0.25\linewidth}{e_0.5-b_100-loss}\\%
    \includeplot{0.25\linewidth}{e_0.2-b_100-loss}%
    \includeplot{0.25\linewidth}{e_0.1-b_100-loss}%
    \caption{In this set of experiments, the training batch size is $b = 100$.}
    \label{fig:experiments-more-100}
\end{figure}

\begin{figure}
    \centering
    \makebox[0.25\linewidth][c]{\footnotesize{}Without privacy noise}%
    \makebox[0.25\linewidth][c]{\footnotesize{}With privacy noise ($\epsilon = 0.5$)}%
    \makebox[0.25\linewidth][c]{\footnotesize{}With privacy noise ($\epsilon = 0.2$)}%
    \makebox[0.25\linewidth][c]{\footnotesize{}With privacy noise ($\epsilon = 0.1$)}\\[0.1mm]%
    \includeplot{0.25\linewidth}{e_inf-b_250}%
    \includeplot{0.25\linewidth}{e_0.5-b_250}\\%
    \includeplot{0.25\linewidth}{e_0.2-b_250}%
    \includeplot{0.25\linewidth}{e_0.1-b_250}\\%
    \includeplot{0.25\linewidth}{e_inf-b_250-loss}%
    \includeplot{0.25\linewidth}{e_0.5-b_250-loss}\\%
    \includeplot{0.25\linewidth}{e_0.2-b_250-loss}%
    \includeplot{0.25\linewidth}{e_0.1-b_250-loss}%
    \caption{In this set of experiments, the training batch size is $b = 250$.}
    \label{fig:experiments-more-250}
\end{figure}

\begin{figure}
    \centering
    \makebox[0.25\linewidth][c]{\footnotesize{}Without privacy noise}%
    \makebox[0.25\linewidth][c]{\footnotesize{}With privacy noise ($\epsilon = 0.5$)}%
    \makebox[0.25\linewidth][c]{\footnotesize{}With privacy noise ($\epsilon = 0.2$)}%
    \makebox[0.25\linewidth][c]{\footnotesize{}With privacy noise ($\epsilon = 0.1$)}\\[0.1mm]%
    \includeplot{0.25\linewidth}{e_inf-b_500}%
    \includeplot{0.25\linewidth}{e_0.5-b_500}\\%
    \includeplot{0.25\linewidth}{e_0.2-b_500}%
    \includeplot{0.25\linewidth}{e_0.1-b_500}\\%
    \includeplot{0.25\linewidth}{e_inf-b_500-loss}%
    \includeplot{0.25\linewidth}{e_0.5-b_500-loss}\\%
    \includeplot{0.25\linewidth}{e_0.2-b_500-loss}%
    \includeplot{0.25\linewidth}{e_0.1-b_500-loss}%
    \caption{In this set of experiments, the training batch size is $b = 500$.}
    \label{fig:experiments-more-500}
\end{figure}
